# Supplementary material for: A first-principles Quantum Monte Carlo study of two-dimensional (2D) GaSe
Source: arXiv:2007.13969 source file (2020-10-21)
Supplement: Supplementary file 1 [file suppinfo_forpub.pdf]

# Supplementary Material: A first-principles Quantum Monte Carlo study of two-dimensional (2D) GaSe

Daniel Wines,† Kayahan Saritas,‡ and Can Ataca*,†

†*Department of Physics, University of Maryland Baltimore County, Baltimore MD 21250*

‡ *Department of Applied Physics, Yale University, New Haven CT 06520*

E-mail: ataca@umbc.edu

## DFT and DMC convergence testing and additional details

Table S1: To verify the pseudopotential conversion, the calculated ionization potential and electron affinity for Ga and Se atoms calculated with the converted plane wave format BFD and ccECP potentials using PBE are given. The experimental values are also given as a reference.

| Method | Ionization Potential (eV) | Electron Affinity (eV) |
|---|---|---|
| PBE (BFD) | Ga: 5.89, Se: 9.44 | Ga: 0.32, Se: 2.15 |
| PBE (ccECP) | Ga: 5.89, Se: 9.51 | Ga: 0.31, Se: 2.17 |
| Exp | Ga: 6.00,[1] Se: 9.75[1] | Ga: 0.30,[2] Se: 2.02[3] |

To convert these Gaussian potentials to plane wave format, we used the ppconvert[4] tool implemented in QMCPACK. We converted these Gaussian potentials to plane wave format and validated this conversion by calculating the ionization potential (IP) and electron affinity (EA) at the DFT level. In addition to these BFD energy-consistent potentials, a new set of

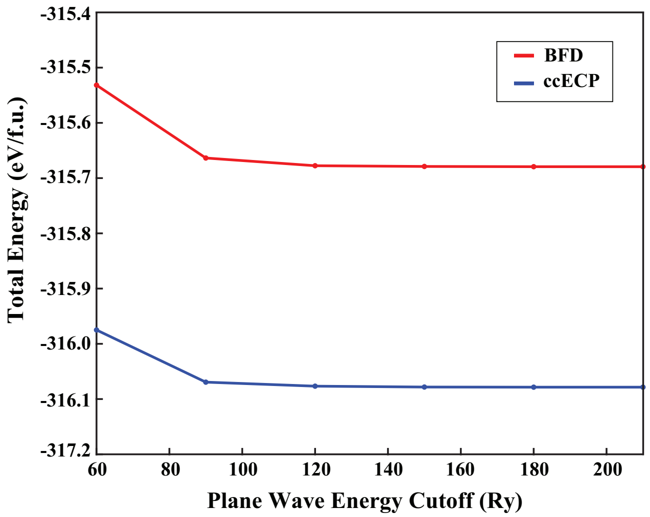


Figure S1: The total energy per formula unit of 2D GaSe as a function of plane wave cutoff energy for the BFD and ccECP potentials (converted to plane wave format) calculated with PBE. The results show a converged value of 120 Ry, which was used for all DFT and QMC calculations.

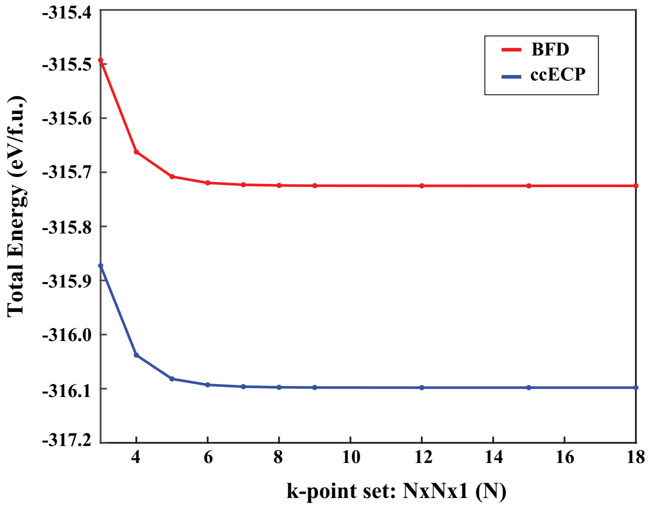


Figure S2: The total energy per formula unit of 2D GaSe as a function of k-point grid for the BFD and ccECP potentials (converted to plane wave format) calculated with PBE. The results show a converged k-point grid of 6x6x1, which was used for all DFT and QMC calculations.

effective core potentials from correlated calculations (ccECP) for Ga and Se have recently been developed specifically for QMC.[5] We also converted these potentials to plane wave format and benchmarked these along with the BFD potentials at the DFT level. We used the d local channel for the BFD potential and the s local channel for the ccECP channel. Since the results of the ccECP and BFD potentials are nearly identical at the DFT level, we decided to use the BFD potentials since the potentials are almost indistinguishable for all calculated properties (at most a 0.13 eV energy difference in cohesive energy, 0.07 eV difference in band gap, 0.06 eV difference for IP and 0.02 eV difference for EA).

For our DFT calculations in VASP, we used standard PBE PAW (as opposed to hard or soft) potentials from version 5.4.4. For the GW-BSE calculations we used standard PBE PAW potentials, specifically designed for GW calculations (also from the VASP 5.4.4 library). The standard PBE potentials were chosen (as opposed to hard/soft or potentials that contain more valence electrons) because they offer a good compromise between accuracy and computational efficiency. The GW-specific PAW potentials are necessary for convergence at the GW-BSE level.

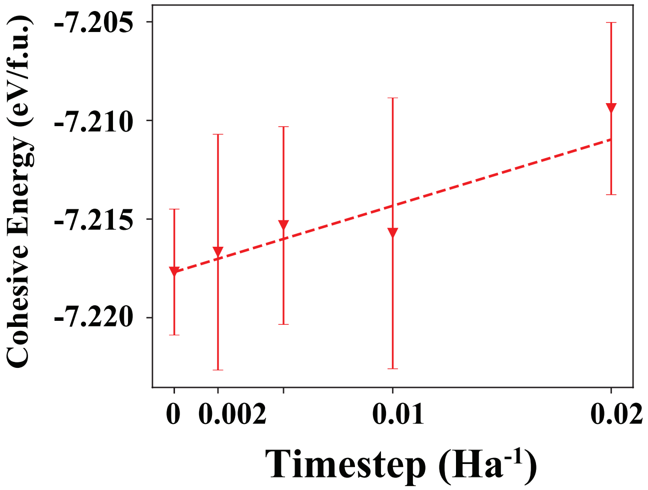


Figure S3: The timestep convergence test for the cohesive energy of monolayer GaSe. A 36 atom cell was used for the convergence testing.

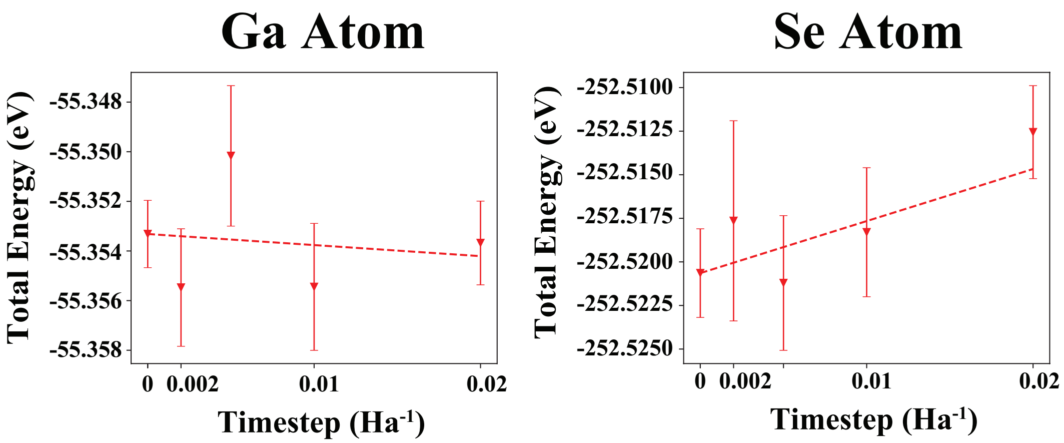


Figure S4: The timestep convergence test for the total energy of a single Ga atom and a single Se atom. The timestep extrapolated values for total energy were used in the calculation of cohesive energy.

Table S2: The cohesive energy per formula unit ($E_{coh}$) and the interlayer binding energy ($E_b$) for 2D GaSe obtained from structural relaxation with each respective DFT functional. Pseudopotential choice is indicated in parenthesis.

| Method | $E_{coh}$ (eV/f.u.) | $E_b$ (eV) |
|---|---|---|
| PBE (PAW) | -6.657 | -0.002 |
| PBE+D2 (PAW) | -7.091 | -0.097 |
| PBE (BFD) | -7.112 | -0.029 |
| PBE+D2 (BFD) | -7.558 | -0.121 |
| PBE (ccECP) | -6.988 | -0.002 |
| PBE+D2 (ccECP) | -7.428 | -0.084 |

# Investigation of Electronic and Optical properties using DFT and DMC

Table S3: The Kohn-Sham electronic gap for 2D GaSe calculated with the relaxed geometry of each respective DFT functional for the Γ-M, Γ-Γ and Γ-K transitions in eV. Pseudopotential choice is indicated in parenthesis.

| | Γ-M | Γ-Γ | Γ-K |
|---|---|---|---|
| *Kohn-Sham eigenstates* | | | |
| PBE (PAW) | 2.277 | 1.919 | 2.718 |
| PBE (BFD) | 2.393 | 2.406 | 2.591 |
| PBE (ccECP) | 2.400 | 2.302 | 2.631 |

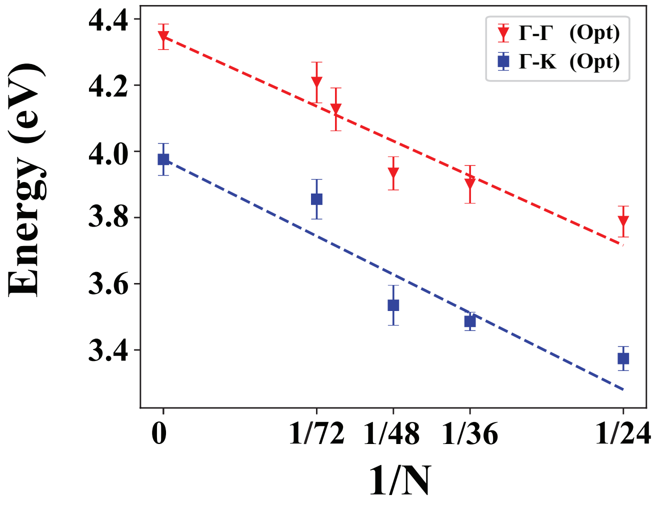


Figure S5: The finite-size scaling of the optical band gap for the Γ-Γ and Γ-K transition. Simulations were performed at N = 72, 48, 36, 24 atoms for both transitions, and also performed at N = 64 for the Γ-Γ transition.

The gap as $N \to \infty$ was extrapolated from the calculated data.

In addition to $G_0W_0$, we solved the Bethe-Salpeter equation (BSE) using $G_0W_0$ as a starting point for PBE and SCAN wavefunctions. From here we were able to obtain the frequency-dependent dielectric function shown in Fig. S7. The first peak of the dielectric function is the optical gap of the material. In addition we calculated the electron-hole coupling strength at each point in the Brillouin zone (BZ) on top of the $G_0W_0$ quasiparticle band structure, shown in Fig. S8.

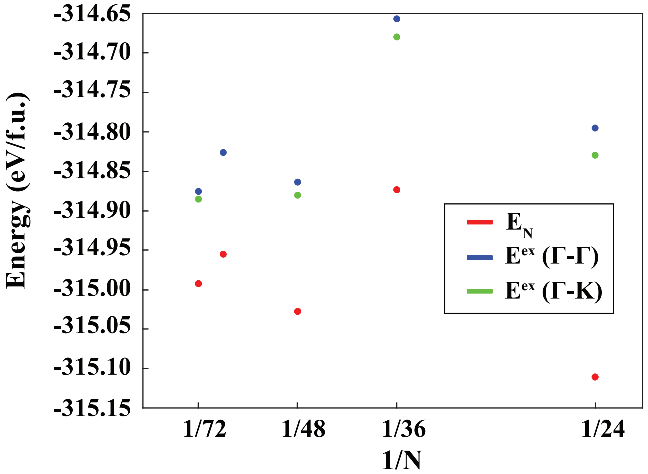


Figure S6: The total energy per formula unit of the neutral GaSe cell (red) and the energy of the Γ-Γ (blue) and Γ-K (green) excited cell as a function of 1/N.

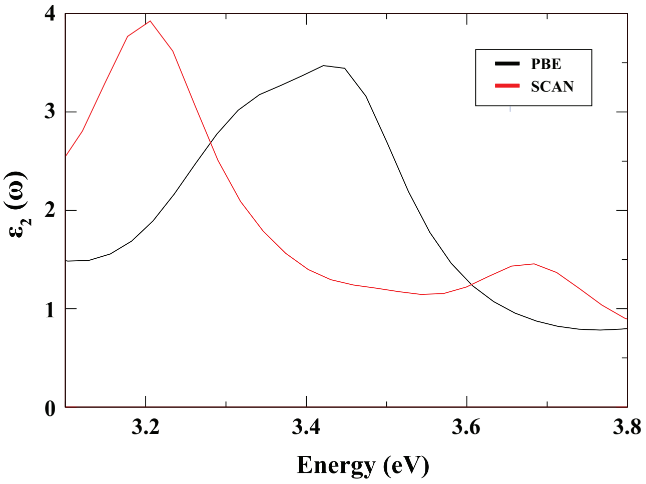


Figure S7: The frequency dependent imaginary part of the dielectric function calculated with BSE using PBE (black) and SCAN (black) wavefunctions using PAW potentials. The first peak shown represents the optical band gap.

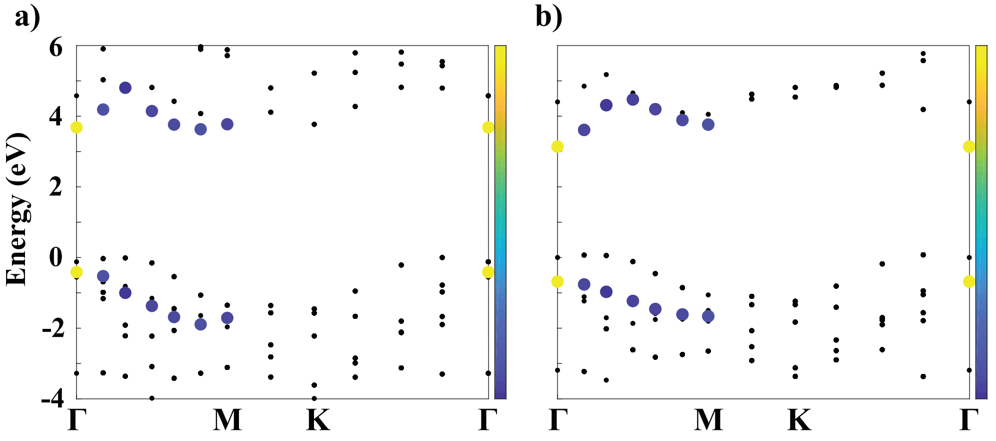


Figure S8: The $G_0W_0$ quasiparticle band structure of GaSe with the fat bands projected on it for a) PBE and b) SCAN wavefunctions (both with PAW potentials). The color represents the contribution of e-h pairs at each point in the Brillouin zone ($|A^1_{c,v,\vec{k}}|$) to the first exciton wavefunction.

The exciton wavefunction can be expressed in an electron-hole product basis, $\Phi^1 = \sum_{c,v,\vec{k}} A^1_{c,v,\vec{k}} \Phi_{c,\vec{k}} \Phi_{v,\vec{k}}$, where $\Phi$ represents an eigenstate in the electron-hole basis, $A$ represents the electron-hole coupling strength, and the indexes $c$, $v$, and $\vec{k}$ represent the conduction band, valence band and specific point in the BZ (see reference[6]). The first eigenstate of the BSE eigenvalue problem, the first exciton peak, can be visualized by plotting $|A^1_{c,v,\vec{k}}|$ as a fat band structure (which was previously demonstrated in[6]). The color axis of Fig. S8 represents the electron-hole coupling strength.

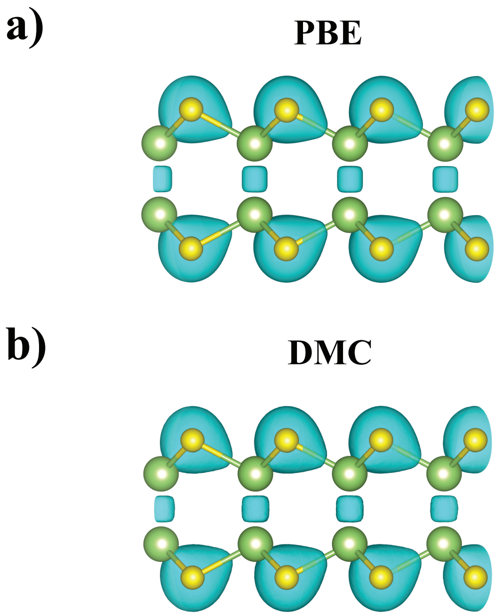


Figure S9: The total ground state charge density of monolayer GaSe calculated with a) DFT (PBE) and b) DMC using BFD pseudopotentials. The isosurface value of both figures were set to 0.05 e/Å$^3$

## References

(1) Lide, D. R. *CRC Handbook of chemistry and physics*; CRC Press, 2008.

(2) Gibson, N. D.; Walter, C. W.; Crocker, C.; Wang, J.; Nakayama, W.; Yukich, J. N.; Eliav, E.; Kaldor, U. Electron affinity of gallium and fine structure of $Ga^-$: Experiment and theory. *Phys. Rev. A* **2019**, *100*, 052512.

(3) Vandevraye, M.; Drag, C.; Blondel, C. Electron affinity of selenium measured by photodetachment microscopy. *Phys. Rev. A* **2012**, *85*, 015401.

(4) Kim, J. et al. QMCPACK: an open sourceab initioquantum Monte Carlo package for the electronic structure of atoms, molecules and solids. **2018**, *30*, 195901.

(5) Wang, G.; Annaberdiyev, A.; Melton, C. A.; Bennett, M. C.; Shulenburger, L.; Mitas, L. A new generation of effective core potentials from correlated calculations: 4s and 4p

main group elements and first row additions. *The Journal of Chemical Physics* **2019**, *151*, 144110.

(6) Bokdam, M.; Sander, T.; Stroppa, A.; Picozzi, S.; Sarma, D. D.; Franchini, C.; Kresse, G. Role of Polar Phonons in the Photo Excited State of Metal Halide Perovskites. *Scientific Reports* **2016**, *6*, 28618.
